# Supplementary material for: Fermion doubling theorems in 2D non-Hermitian systems for Fermi points and exceptional points
Source: arXiv:1912.02788 source file (2020-12-18)
Supplement: Supplementary file 1 [file SM.pdf]

# Note for the “Two fold non-Hermitian degeneracy points”

Zhesen Yang<sup>1,2</sup>

<sup>1</sup>Beijing National Laboratory for Condensed Matter Physics,  
Institute of Physics, Chinese Academy of Sciences, Beijing 100190, China

<sup>2</sup>University of Chinese Academy of Sciences, Beijing 100049, China

(Dated: December 12, 2019)

PACS numbers:

## I. TWO-FOLD NON-HERMITIAN DEGENERACY POINTS

Consider the following two-band Hamiltonian,

$$\mathcal{H}(\mathbf{k}) = h_x(\mathbf{k})\sigma_x + h_y(\mathbf{k})\sigma_y + h_z(\mathbf{k})\sigma_z, \quad (1)$$

where  $h_{x/y/z}(\mathbf{k}) = h_{x/y/z}^r(\mathbf{k}) + ih_{x/y/z}^i(\mathbf{k})$  are complex functions of  $\mathbf{k}$ . The band degeneracy at  $\mathbf{k}_0$  requires the vanishing of the discriminant of the characteristic polynomial, namely

$$\Delta_f(\mathbf{k}_0) = h_x^2(\mathbf{k}_0) + h_y^2(\mathbf{k}_0) + h_z^2(\mathbf{k}_0) = 0. \quad (2)$$

In order to analysis the winding number of the degenerate point  $\mathbf{k}_0$ , we can expand the Hamiltonian as follows

$$\begin{aligned} h_x(\mathbf{k}_0 + \delta\mathbf{k}) &\simeq c_x + c_{x,x}\delta k_x + c_{x,y}\delta k_y + c_{x,xx}\delta k_x^2 + c_{x,xy}\delta k_x\delta k_y + c_{x,yy}\delta k_y^2 + \dots, \\ h_y(\mathbf{k}_0 + \delta\mathbf{k}) &\simeq c_y + c_{y,x}\delta k_x + c_{y,y}\delta k_y + c_{y,xx}\delta k_x^2 + c_{y,xy}\delta k_x\delta k_y + c_{y,yy}\delta k_y^2 + \dots, \\ h_z(\mathbf{k}_0 + \delta\mathbf{k}) &\simeq c_z + c_{z,x}\delta k_x + c_{z,y}\delta k_y + c_{z,xx}\delta k_x^2 + c_{z,xy}\delta k_x\delta k_y + c_{z,yy}\delta k_y^2 + \dots, \end{aligned} \quad (3)$$

where all the coefficients are complex numbers.

### A. Zeroth order

Up to the zeroth order of  $h_{x/y/z}(\mathbf{k})$ , the Hamiltonian can be written as

$$\mathcal{H}(\mathbf{k}_0) = \begin{pmatrix} c_z & c_x - ic_y \\ c_x + ic_y & -c_z \end{pmatrix}. \quad (4)$$

The band degeneracy requires

$$\Delta_f(\mathbf{k}_0) = 0; \quad \text{or} \quad c_x^2 + c_y^2 + c_z^2 = 0. \quad (5)$$

The band degeneracy can be further classified as EP and non-EP. The condition of non-EP is

$$\begin{aligned} \text{non-EP} : \mathbf{h}(\mathbf{k}_0) &= (h_x(\mathbf{k}_0), h_y(\mathbf{k}_0), h_z(\mathbf{k}_0)) = 0, \quad \text{or} \quad \mathbf{c} = (c_x, c_y, c_z) = 0; \\ \text{EP} : \Delta_f(\mathbf{k}_0) &= 0 \cap \mathbf{h}(\mathbf{k}_0) \neq 0, \quad \text{or} \quad c_x^2 + c_y^2 + c_z^2 = 0 \cap \mathbf{c} \neq 0. \end{aligned} \quad (6)$$

Thus one can notice that the number of constraint equations (NCE) for EP is 2 and for non-EP is 6.

### B. First order

#### 1. EP

Up to the first order of  $h_{x/y/z}(\mathbf{k})$ , the discriminant can be written as

$$\begin{aligned} \text{EP} : \Delta_f(\mathbf{k}_0) &\simeq (c_x + c_{x,x}\delta k_x + c_{x,y}\delta k_y)^2 + (c_y + c_{y,x}\delta k_x + c_{y,y}\delta k_y)^2 + (c_z + c_{z,x}\delta k_x + c_{z,y}\delta k_y)^2 \\ &\simeq (c_x c_{x,x} + c_y c_{y,x} + c_z c_{z,x})\delta k_x + (c_x c_{x,y} + c_y c_{y,y} + c_z c_{z,y})\delta k_y \\ &:= (C_x^r + iC_x^i)\delta k_x + (C_y^r + iC_y^i)\delta k_y \end{aligned} \quad (7)$$

Now we define

$$\det[C] := \begin{pmatrix} C_x^i & C_y^i \\ C_x^r & C_y^r \end{pmatrix}. \quad (8)$$

Then, according to the definition of the winding number

$$\nu_E(\mathbf{K}_0) = \frac{i}{2\pi} \oint_{\Gamma(\mathbf{K}_0)} d\mathbf{k} \cdot \nabla_{\mathbf{k}} (\ln \det[h(\mathbf{k})]), \quad (9)$$

if  $\det[C] \neq 0$ , one can show that

$$\nu_E(\mathbf{K}_0) = \det[C]. \quad (10)$$

On the other hand, if  $\det[C] = 0$ , the winding number must be zero.

## 2. non-EP

For the non-EP, the discriminant does not have liner term,

$$\text{non-EP} : \Delta_f(\mathbf{k}_0) \simeq (c_{x,x}\delta k_x + c_{x,y}\delta k_y)^2 + (c_{y,x}\delta k_x + c_{y,y}\delta k_y)^2 + (c_{z,x}\delta k_x + c_{z,y}\delta k_y)^2. \quad (11)$$

## II. HIGH ORDER

### 1. EP

Up to the second order, the winding number can be  $\pm 2$ , which requires

$$\text{EP}(\nu = \pm 2) : C_x^r = C_x^i = C_y^r = C_y^i = 0 \quad (12)$$

Thus additional 4 independent parameters are required to be zero. Generalize the above discussion, one can obtain

$$\text{EP}(\nu = \pm 3) : C_{xx}^r = C_{xx}^i = C_{xy}^r = C_{xy}^i = C_{yy}^r = C_{yy}^i = 0 \quad (13)$$

### 2. non-EP

For the non-EP, we have

$$\begin{aligned} \text{non-EP} : \Delta_f(\mathbf{k}_0) &\simeq (c_{x,x}\delta k_x + c_{x,y}\delta k_y + c_{x,xx}\delta k_x^2 + c_{x,xy}\delta k_x\delta k_y + c_{x,yy}\delta k_y^2 + \dots)^2 \\ &+ (c_{y,x}\delta k_x + c_{y,y}\delta k_y + c_{y,xx}\delta k_x^2 + c_{y,xy}\delta k_x\delta k_y + c_{y,yy}\delta k_y^2 + \dots)^2 \\ &+ (c_{z,x}\delta k_x + c_{z,y}\delta k_y + c_{z,xx}\delta k_x^2 + c_{z,xy}\delta k_x\delta k_y + c_{z,yy}\delta k_y^2 + \dots)^2 \\ &\simeq C_{xx}\delta k_x^2 + C_{xy}\delta k_x\delta k_y + C_{yy}\delta k_y^2 + C_{xxx}\delta k_x^3 + C_{xxy}\delta k_x^2\delta k_y + C_{xyy}\delta k_x\delta k_y^2 + C_{yyy}\delta k_y^3 + \dots \end{aligned} \quad (14)$$

Thus

$$\begin{aligned} \text{non-EP}(\nu = 0, \pm 2) : c_x = c_y = c_z = 0 \\ \text{non-EP}(\nu = 1, \pm 3) : C_{xx}^r = C_{xx}^i = C_{xy}^r = C_{xy}^i = C_{yy}^r = C_{yy}^i = 0 \end{aligned} \quad (15)$$

Examples of non-EP

$$\nu = \pm 2 \rightarrow c_x = c_y = c_z = 0 \rightarrow 2 \times 3 = 6$$

$$\nu = \pm 3 \rightarrow c_x = c_y = c_z = C_{xx} = C_{xy} = C_{yy} = 0 \rightarrow 2 \times 3 + 2 \times 3 = 12$$

$$\nu = \pm 4 \rightarrow c_x = c_y = c_z = C_{xx} = C_{xy} = C_{yy} = C_{xxx} = C_{xxy} = C_{xyy} = C_{yyy} = 0 \rightarrow 2 \times 3 + 2(3 + 4) = 20$$

$$\nu = \pm 5 \rightarrow 2 \times 3 + 2(3 + 4 + 5) = 30$$

Thus  $6 + 2n(n+1)/2 - 2(1+2) = n(n+1)$

TABLE I: Two-fold non-Hermitian degenerate points

| EP/non-EP | Winding number $\nu$ | Evolution under perturbations | Minimal stable dimensions |
|-----------|----------------------|-------------------------------|---------------------------|
| EP        | 0                    | Split/Gapped                  | 3                         |
| EP        | $\pm 1$              | Stable                        | 2                         |
| EP        | $\pm n(n \geq 2)$    | Split                         | $n(n + 1)$                |
| non-EP    | 0                    | Split/Gapped                  | 6                         |
| non-EP    | $\pm 1$              | Split                         | 12                        |
| non-EP    | $\pm n(n \geq 2)$    | Split                         | $n(n + 1)$                |
